# Supplementary material for: Investigating Forgetting in Pre-Trained Representations Through Continual Learning
Source: arXiv:2305.05968 source file (2023-05-10)
Supplement: Supplementary file 1 [file appendix.tex]

\appendix

\section{Probing Task Details}
\label{sec:appendix}
